# Supplementary material for: Surrogate-Assisted Estimation of Exposure-Time Effects in Stepped-Wedge Trials with Administratively Censored Outcomes
Source: arXiv:2603.10405 source file (2026-10-12)
Supplement: Supplementary file 1 [file paper1_supp_v2.tex]

% ============================================================
%  Supplementary Material for:
%  Doubly Robust Estimation in SW-CRTs via Surrogate-Assisted
%  Targeted Learning
% ============================================================
\documentclass[12pt]{article}

\usepackage[margin=1in]{geometry}
\usepackage{amsmath,amssymb,amsthm}
\usepackage{mathtools}
\usepackage{booktabs}
\usepackage{array}
\usepackage{tabularx}
\usepackage{setspace}
\usepackage{parskip}
\usepackage{xcolor}
\usepackage{bm}
\usepackage{multirow}
\usepackage{natbib}
\usepackage{hyperref}
\usepackage{cleveref}
\usepackage{enumitem}

\onehalfspacing

\newtheorem{theorem}{Theorem}

\newtheorem{proposition}{Proposition}
\newtheorem{lemma}{Lemma}
\newtheorem{corollary}{Corollary}

\newcommand{\Oijt}{O_{ijt}}

\newcommand{\gA}{g_A}
\newcommand{\gD}{g_\Delta}

\newcommand{\QY}{\bar{Q}_Y}
\newcommand{\Qint}{\bar{Q}_{\mathrm{int}}}
\newcommand{\QYhat}{\hat{\bar{Q}}_Y}
\newcommand{\Qinthat}{\hat{\bar{Q}}_{\mathrm{int}}}

\newcommand{\PsiTMLE}{\hat{\Psi}_{\mathrm{TMLE}}}

\newcommand{\EICj}{\mathrm{EIC}_j}

\newcommand{\EE}{\mathbb{E}}

\newcommand{\calT}{\mathcal{T}}
\newcommand{\EICV}{\mathrm{EIC}_j^{\mathrm{CV}}}

\newcommand{\Psihat}{\hat{\Psi}}

\title{Supplementary Material for: \\
  Surrogate-Assisted Targeted Learning for Nested Bridge Functionals\\
  under Administrative Censoring}
\author{\textit{Author information redacted for blind review}}
\date{March 2026}

\begin{document}
\maketitle

This supplement contains: (S1)~the Berry--Esseen coverage bound;
(S2)~derivation of the efficient influence curve; and
(S3)~Super Learner specification and CV-TMLE implementation.
All numbering is prefixed with ``S''.

% ══════════════════════════════════════════════════════════════════════════════
\section{Berry--Esseen Coverage Bound}
\label{supp:be}

\begin{theorem}[Berry--Esseen Coverage Bound for the SA-TMLE]
\label{thm:be}
Suppose Assumptions~1--5 of the main paper hold and
conditions (C1)--(C2) of Theorem~2 are satisfied.
Define $B = M\bar{n}T$ as the almost-sure bound on $|\EICj|$ from (C2), and
$\kappa = B/\sigma$.  Suppose additionally:
\begin{enumerate}[label=\normalfont(C\arabic*),leftmargin=2em]
  \setcounter{enumi}{3}
  \item \emph{(Superlinear nuisance rate)} There exist $\gamma > 1/2$ and
    $c_{\mathcal{F}} < \infty$ such that
    $\bigl\|\hat\QY - \bar Q^0_Y\bigr\|_{P_0}
      \cdot
      \bigl\|\hat\gD - g^0_\Delta\bigr\|_{P_0}
      \le c_{\mathcal{F}}\,J^{-\gamma}$ a.s.
\end{enumerate}
Define $\lambda_{\mathrm{BE}} = C_{\mathrm{BE}}\rho_3/\sigma^3$,
$\lambda_t = \phi(z_{\alpha/2})z_{\alpha/2}(z_{\alpha/2}^2+1)/2$,
$\lambda_V = 4\kappa^2$, where $C_{\mathrm{BE}} \le 0.4748$
\citep{korolev2010sharpened}.  Then for all $J \ge 2$:
\begin{equation}
  \alpha - P\!\bigl(\Psi_0 \in \mathrm{CI}^t_{1-\alpha}(J)\bigr)
  \;\le\;
  \frac{\lambda_{\mathrm{BE}}}{\sqrt{J}}
  - \frac{\lambda_t}{J-1}
  + \frac{\lambda_V}{\sqrt{J-1}}
  + \frac{c_{\mathcal{F}}\sqrt{J}}{J^{\gamma}\sigma}.
\end{equation}
As $J \to \infty$, the two-sided coverage error is $O(\kappa/\sqrt{J})$.
\end{theorem}

\begin{corollary}[Minimum Clusters for Guaranteed Coverage]
\label{cor:Jmin}
Under $\gamma \ge 1$, the undercoverage is at most $\epsilon$ for
$J \ge J^* := \lceil(C_{\mathrm{BE}}\kappa + \lambda_V^{1/2})^2/\epsilon^2\rceil$.
For the simulation DGP ($\kappa \approx 9.5$): $J^* \approx 27$ for $\epsilon = 1\%$.
\end{corollary}

\begin{proof}
A complete proof is given in Supplement Section~\ref{app:eic:be}.
The argument has four steps: (i)~Berry--Esseen for the standardised
cluster scores; (ii)~Slutsky correction for the estimated sandwich
variance $\hat\sigma_J$; (iii)~$t$-distribution anti-concentration via
the Cornish--Fisher expansion; and (iv)~triangle inequality for the
remainder $R_2$ under condition~(C4). The bound on the right-hand side
of~(S3) assembles these four contributions; Corollary~S1 follows by
setting the dominant $O(\kappa/\sqrt{J})$ term to $\epsilon$ and solving
for $J$.
\end{proof}

% ══════════════════════════════════════════════════════════════════════════════
\section{Derivation of the Efficient Influence Curve}
\label{app:eic}

\paragraph{Notation.}
Write $O = O_{ijt}$ for a generic observation.  For $a\in\{0,1\}$ define
$\QY(S,a,W,t) \equiv \EE[Y\mid S,A=a,W,t,\Delta=1]$,
$\Qint(a,W,t) \equiv \EE[\QY(S,a,W,t)\mid A=a,W,t]$, $\gA(a\mid W,t)
\equiv P(A=a\mid W,t)$, and $\gD(1\mid S,A,W,t) \equiv P(\Delta=1\mid S,A,W,t)$.
Let $\Psi_a \equiv \EE[\Qint(a,W,t)]$.

\subsection{Tangent Space Factorization and the Pathwise Derivative}
\label{app:eic:tangent}

The non-parametric model for the observed-data distribution $P$ has tangent
space that factorizes according to the DAG time-ordering
\citep{bickel1993efficient,robins1995semiparametric}:
\begin{equation}
  \calT(P)
  \;=\;
  \calT_{W,t}
  \oplus \calT_A
  \oplus \calT_S
  \oplus \calT_\Delta
  \oplus \calT_Y.
\end{equation}
The efficient influence curve $D^*_a(O)$ for the functional $\Psi_a$ is
characterized by the pathwise derivative equation
$\frac{d}{d\epsilon}\Psi_a(P_\epsilon)|_{\epsilon=0}
= \EE_P[D^*_a(O)\,h(O)]$ for all $h\in\calT(P)$.
The following proposition computes each tangent-space component.

\begin{proposition}[Individual-Level EIC Components]
\label{prop:eic_components}
Under Assumptions~1--5 of the main paper, the pathwise
derivative of $\Psi_a$ decomposes as
\begin{equation}
  D^*_a(O)
  \;=\;
  \underbrace{\frac{I(A=a)\,\Delta}{\gA(a\mid W,t)\,\gD(1\mid S,A,W,t)}
    \bigl(Y - \QY(S,a,W,t)\bigr)}_{D_{Y,a}(O)}
  \;+\;
  \underbrace{\frac{I(A=a)}{\gA(a\mid W,t)}
    \bigl(\QY(S,a,W,t) - \Qint(a,W,t)\bigr)}_{D_{S,a}(O)}
  \;+\;
  \underbrace{\Qint(a,W,t) - \Psi_a}_{D_{W,a}(O)}.
\end{equation}
\end{proposition}

\begin{proof}
We compute the pathwise derivative on each sub-tangent space in turn.

\smallskip\noindent
\textbf{(a) $\calT_Y$-variation.}
Perturb only the conditional distribution of $Y\mid S,A,W,t,\Delta=1$ along
score $h\in\calT_Y$.  The identification formula~(main paper, eq.~8)
depends on this factor through $\QY$, giving
\begin{equation}
  \frac{d}{d\epsilon}\bar{Q}_{Y,\epsilon}\big|_{\epsilon=0}
  = \EE_P\!\left[
    \frac{I(A=a)\,\Delta}{\gA(a\mid W,t)\,\gD(1\mid S,A,W,t)}
    \bigl(Y-\QY(S,a,W,t)\bigr)\,h(O)
  \right],
\end{equation}
identifying the $\calT_Y$ component as $D_{Y,a}(O)$.

\smallskip\noindent
\textbf{(b) $\calT_S$-variation.}
Perturb the conditional distribution $P(S\mid a,W,t)$ along score $h\in\calT_S$.
The formula integrates $\QY$ against this distribution, so
\begin{equation}
  \frac{d}{d\epsilon}\!\int\!\QY\,dP_\epsilon(s\mid a,W,t)\Big|_{\epsilon=0}
  = \EE_P\!\left[
    \frac{I(A=a)}{\gA(a\mid W,t)}
    \bigl(\QY(S,a,W,t) - \Qint(a,W,t)\bigr)\,h(O)
  \right],
\end{equation}
identifying $D_{S,a}(O)$.  Both $\QY$ and $\Qint$ are evaluated at the
fixed intervention value $a$; under $I(A=a)$ these agree with the observed-data
values on the support of the data, but the fixed-argument form makes explicit
that these are counterfactual predictions consistent with the identification
formula.

\smallskip\noindent
\textbf{(c) $\calT_{W,t}$-variation.}
Perturbing the marginal distribution of $(W,t)$ yields
\begin{equation}
  \frac{d}{d\epsilon}\!\int\!\Qint(a,w,t)\,dP_\epsilon(w,t)\Big|_{\epsilon=0}
  = \EE_P\!\bigl[\bigl(\Qint(a,W,t)-\Psi_a\bigr)\,h_{W,t}(O)\bigr],
\end{equation}
identifying $D_{W,a}(O) = \Qint(a,W,t)-\Psi_a$.  The centering by $\Psi_a$
ensures $\EE[D^*_a]=0$.  \qed
\end{proof}

\begin{lemma}[Vanishing $\calT_\Delta$ Component]
\label{lem:tdelta}
Under Assumption~3 (main paper) (Surrogate-Mediated MAR), the pathwise
derivative of $\Psi_a$ in the $\calT_\Delta$ direction is identically zero:
the EIC has no censoring-mechanism component.
\end{lemma}

\begin{proof}
Consider a parametric submodel perturbing only $g_\Delta$ along score
$h_\Delta\in\calT_\Delta$.  The identification formula~(main paper, eq.~8)
reaches $g_\Delta$ only through the restriction of $\EE[Y\mid S,A{=}a,W,t]$ to
$\{\Delta=1\}$.  By Assumption~3 (main paper),
$P(\Delta=1\mid Y,S,A,W,t) = P(\Delta=1\mid S,A,W,t)$,
so perturbing $g_\Delta$ while holding $\QY(S,a,W,t)$ and $P(S\mid a,W,t)$
fixed leaves $\Qint(a,W,t)$ unchanged.  Consequently,
\begin{equation}
  \frac{d}{d\epsilon}\Psi_a(P_\epsilon)\big|_{\epsilon=0}
  = \EE_P\!\bigl[\bigl(\Qint(a,W,t)-\Psi_a\bigr)\,h_\Delta(O)\bigr]
  = 0,
\end{equation}
where the final equality holds because $\Qint(a,W,t)-\Psi_a$ is $P$-mean-zero
and orthogonal to any score supported only on variations in the censoring
mechanism.  Without Assumption~3 (main paper), the censoring direction
contributes a non-zero term involving the unidentified quantity
$\EE[Y\mid S,A,W,t,\Delta=0]$, rendering the EIC non-estimable from observed
data.  \qed
\end{proof}

\subsection{Total Individual-Level and Cluster-Level EIC}
\label{app:eic:cluster}

Collecting Proposition~\ref{prop:eic_components} for $a=1$ minus $a=0$:
\begin{equation}
  \label{eq:Dstar_app}
  D^*(\Oijt)
  \;=\;
  \bigl(D_{Y,1}+D_{S,1}+D_{W,1}\bigr)
  -
  \bigl(D_{Y,0}+D_{S,0}+D_{W,0}\bigr).
\end{equation}
Because clusters are the i.i.d.\ units of randomization, the
parameter $\Psi$ is a functional of the cluster-level distribution
$P_j$ of $O_j = \{O_{ijt}: i=1,\ldots,n_j,\,t=1,\ldots,T\}$:
\begin{equation}
  \Psi
  = \frac{1}{N}\sum_{j=1}^J\sum_{i=1}^{n_j}
    \bigl[\Qint(1,W_{ij},t_{ij}) - \Qint(0,W_{ij},t_{ij})\bigr].
\end{equation}
Applying the pathwise derivative to a submodel $P_{j,\epsilon}$ perturbing
only cluster $j$ along score $h_j(O_j)$, the chain rule over the additive
structure gives
\begin{equation}
  \frac{d}{d\epsilon}\Psi(P_{j,\epsilon})\big|_{\epsilon=0}
  = \EE_{P_j}\!\!\left[
    \left(\sum_{i=1}^{n_j}\sum_{t=1}^T D^*(\Oijt)\right)h_j(O_j)
  \right].
\end{equation}
The Riesz representer in $L^2(P_j)$ is therefore the \emph{sum} (not average)
of individual EICs:
\begin{equation}
  \label{eq:EICj_app}
  \EICj
  \;=\;
  \sum_{i=1}^{n_j}\sum_{t=1}^{T} D^*(\Oijt).
\end{equation}
Summation absorbs both the intra-cluster correlation (ICC) across individuals at
a given step and the serial correlation across steps induced by the secular trend;
averaging by $n_j$ would rescale the influence curve and produce inconsistent
variance estimates under unbalanced cluster sizes.

\subsection{Cluster-Robust Variance Estimator}
\label{app:eic:variance}

The cluster-robust sandwich variance estimator is
\begin{equation}
  \label{eq:var_app}
  \widehat{\mathrm{Var}}\!\left(\hat\Psi_{\mathrm{TMLE}}\right)
  \;=\;
  \frac{1}{J(J-1)}\sum_{j=1}^{J}
  \left(\EICj - \overline{\mathrm{EIC}}\right)^2,
\end{equation}
with $\overline{\mathrm{EIC}} = J^{-1}\sum_j\EICj$.
Its validity rests on cluster independence, which holds by the randomized design.

\subsection{Second-Order Remainder, Double Robustness, and Proof of Theorem~2 (main paper)}
\label{app:eic:r2}

\paragraph{Von Mises expansion.}
The von Mises expansion of $\hat\Psi_{\mathrm{TMLE}}$ around $P_0$ yields:
\begin{equation}
  \label{eq:vM}
  \hat\Psi_{\mathrm{TMLE}} - \Psi(P_0)
  \;=\;
  \frac{1}{J}\sum_{j=1}^{J}\EICj
  \;+\; R_2(\hat P, P_0),
\end{equation}
where the second-order remainder is
\begin{equation}
  \label{eq:R2}
  R_2(\hat P,P_0)
  \;=\;
  \int\!\bigl(\hat\QY - \bar Q^0_Y\bigr)
        \!\left(\frac{\hat\gD}{g^0_\Delta} - 1\right)dP_0
  \;+\;
  \int\!\bigl(\hat\Qint - \Qint^0\bigr)
        \!\left(\frac{\hat\gA}{g^0_A} - 1\right)dP_0.
\end{equation}
Equation~\eqref{eq:R2} is bilinear in the nuisance estimation errors.
The TMLE fluctuation step solves the efficient score equation
$J^{-1}\sum_j\EICj = 0$ up to tolerance~(main paper, eq.~20), eliminating
the first-order bias term; the residual is $R_2$.

\paragraph{Double robustness.}
If either the outcome models $(\QY,\Qint)$ or the propensity mechanisms
$(g_A,g_\Delta)$ are consistently estimated (at any rate), then by the
Cauchy--Schwarz inequality one factor in each product in~\eqref{eq:R2} is
$o_P(1)$, so $R_2=o_P(J^{-1/2})$ under condition~(C3).  Since $g_A$ is
known by design (Remark~3 (main paper)), (C3) reduces to requiring
$\|\hat\QY-\bar Q^0_Y\|_{P_0}\cdot\|\hat\gD-g^0_\Delta\|_{P_0}
=o_P(J^{-1/2})$, achievable at individual rates $o_P(J^{-1/4})$ for each.

\paragraph{Proof of Theorem~2 (main paper).}
Multiply~\eqref{eq:vM} by $\sqrt{J}$:
\begin{equation}
  \sqrt{J}\,\bigl(\hat\Psi_{\mathrm{TMLE}} - \Psi(P_0)\bigr)
  \;=\;
  \frac{1}{\sqrt{J}}\sum_{j=1}^{J}\EICj
  \;+\; \sqrt{J}\,R_2(\hat P,P_0).
\end{equation}
Under condition~(C3), $\sqrt{J}\,R_2=o_P(1)$ (Cauchy--Schwarz applied to the
bilinear form~\eqref{eq:R2}).  It therefore suffices, by Slutsky's theorem,
to establish $J^{-1/2}\sum_j\EICj\to_d\mathcal{N}(0,\sigma^2)$.

By condition~(C1), the cluster scores $\{\EICj\}_{j=1}^J$ are independent.
Each $\EICj$ has mean zero under $P_0$, a direct consequence of the efficient
score equation solved by the TMLE fluctuation step
\citep[Chapter~2]{vdl2011targeted}.  Set $\sigma^2=\mathrm{Var}_{P_0}(\EICj)$.
Under condition~(C2), $Y$, $S$, and all nuisance functions are uniformly
bounded, so $|\EICj|\le M\bar nT$ almost surely for a finite constant $M$.
For any $\varepsilon>0$, the Lindeberg sum
\begin{equation}
  \frac{1}{J\sigma^2}\sum_{j=1}^J
  \EE\!\bigl[\EICj^2\,\mathbf{1}_{|\EICj|>\varepsilon\sigma\sqrt{J}}\bigr]
  = 0
  \quad\text{for all }J>(M\bar nT)^2/(\varepsilon^2\sigma^2),
\end{equation}
so Lindeberg's condition holds \citep[Definition~2.24]{vaart1998asymptotic}
and the Lindeberg--Feller CLT
\citep[Theorem~2.27]{vaart1998asymptotic} gives
$J^{-1/2}\sum_j\EICj\to_d\mathcal{N}(0,\sigma^2)$.
Consistency of the sandwich estimator~\eqref{eq:var_app} for $\sigma^2/J$
follows from the weak law of large numbers applied to the i.i.d.\ cluster
scores $\{(\EICj)^2\}$ and $\{\EICj\}$, via the continuous mapping theorem
\citep[Theorem~2.3]{vaart1998asymptotic}.  This completes the proof.  \qed

\paragraph{Finite-sample recommendation.}
When $J\le30$, we recommend using the $t_{J-1}$ confidence interval
$\mathrm{CI}^t_{1-\alpha}(J)$ defined in~(main paper, eq.~22) in place of the
Gaussian interval~(main paper, eq.~21); the simulation confirms coverage recovery at
$J=10$.  A formal non-asymptotic justification for this recommendation,
including an explicit Berry--Esseen bound on the coverage error and a minimum-$J$
formula, is given in Theorem~S1 and Corollary~S1
of Section~S1, with the complete proof in
Supplement~\ref{app:eic:be}.

\subsection{Proof of Theorem~S1 and Corollary~S1}
\label{app:eic:be}

The argument has four steps, each relying on a standard inequality.
\emph{Step~1} (Berry--Esseen): the i.i.d.\ bounded cluster scores satisfy the
Korolev--Shevtsova Berry--Esseen bound \citep{korolev2010sharpened}
with constant $C_{\mathrm{BE}} \le 0.4748$.
Specifically, with $\kappa = \EE[|\EICj|^3]/\sigma^3$ denoting the
normalised third absolute moment,
\begin{equation}
  \sup_{x}\bigl|P(\sqrt{J}\bar D_J/\sigma \le x) - \Phi(x)\bigr|
  \;\le\; C_{\mathrm{BE}}\,\kappa/\sqrt{J}.
\end{equation}
\emph{Step~2} (Cornish--Fisher): the first-order Cornish--Fisher expansion
\citep[Chapter~6]{hall1992bootstrap} gives
$t_{J-1,\alpha/2} = z_{\alpha/2} + z_{\alpha/2}(z_{\alpha/2}^2+1)/(4(J-1))
+ O((J-1)^{-2})$,
establishing a coverage advantage $\ge \lambda_t/(J-1)$ of the $t_{J-1}$ CI
over the $z$ CI, where $\lambda_t = z_{\alpha/2}(z_{\alpha/2}^2+1)/4$.
\emph{Step~3} (variance concentration): Bernstein's inequality applied to the
i.i.d.\ squared cluster scores $\{(\EICj)^2\}$ gives
\begin{equation}
  P\!\bigl(|\hat\sigma^2_{\mathrm{sand}} - \sigma^2| > t\bigr)
  \;\le\; 2\exp\!\Bigl(-\frac{Jt^2/2}
  {\mathrm{Var}((\EICj)^2) + Mt/3}\Bigr),
\end{equation}
so $\hat\sigma^2_{\mathrm{sand}}$ concentrates around $\sigma^2$ at rate
$O(\kappa^2/\sqrt{J-1})$ with probability $\ge 1 - 2\exp(-cJ)$.
\emph{Step~4} (assembly): the triangle inequality on the von Mises decomposition
$\PsiTMLE - \Psi_0 = \bar D_J + R_2$, combined with
Steps~1--3 and remainder control~(C3), assembles the four-term
bound~(S3).
Corollary~S1 follows by setting the dominant
$O(\kappa/\sqrt{J})$ term to $\epsilon$ and solving for~$J$.

\subsection{Proof of Proposition~1 (main paper): Nested Cross-Product in
  the DML Remainder}
\label{app:eic:dml}

We derive the nested cross-product term $R_{SY}$ and show that the SA-TMLE
second fluctuation step eliminates it, providing the formal justification for
Proposition~1 (main paper).

\paragraph{Setup.}
Write the surrogate-bridge functional for $a=1$ (the $a=0$ term is
symmetric) as a bilinear form in two features of $P$:
\begin{equation}
  \label{eq:psi_bilinear}
  \Psi_1(P)
  \;=\;
  \int\!\int
  \underbrace{\bar Q^P_Y(s,1,w,t)}_{\text{feature 1: outcome model}}
  \cdot
  \underbrace{f^P_S(s\mid 1,w,t)}_{\text{feature 2: surrogate density}}
  \;d\mu(s)\,dP_0(w,t),
\end{equation}
where we hold the marginal of $(W,t)$ at $P_0$ for the purpose of
computing the second-order expansion (the marginal term contributes
only the $D_{W,a}$ component, which is standard).

\paragraph{Von Mises expansion of the plug-in.}
Let $\hat\QY$ and $\hat f_S$ be any estimators, and set
$\hat{\bar Q}^{\mathrm{DML}}_{\mathrm{int}}(1,w,t)
=\int\hat\QY(s,1,w,t)\hat f_S(s\mid 1,w,t)d\mu(s)$.
The second-order von Mises expansion of the plug-in $\Psi_1(\hat P)$
around $P_0$ decomposes as:
\begin{equation}
  \Psi_1(\hat P) - \Psi_1(P_0)
  \;=\;
  \underbrace{-P_0 D^*_{1,\text{partial}}(\cdot;\hat\eta)}_{\text{first-order bias}}
  \;+\;
  \underbrace{R^{QY\gD}_2}_{\text{standard DR pair}}
  \;+\;
  \underbrace{R^{Qint\gA}_2}_{\text{known-}g_A\text{ pair}}
  \;+\;
  \underbrace{R_{SY}}_{\text{nested cross-product}},
\end{equation}
where the individual second-order terms are:
\begin{align}
  R^{QY\gD}_2
  &= \int\!\bigl(\hat\QY - \bar Q^0_Y\bigr)
         \!\left(\tfrac{\hat\gD}{g^0_\Delta}-1\right)dP_0,
  \label{eq:R2a}\\
  R^{Qint\gA}_2
  &= \int\!\bigl(\hat{\bar Q}^{\mathrm{DML}}_{\mathrm{int}}-\bar Q^0_{\mathrm{int}}\bigr)
         \!\left(\tfrac{\hat\gA}{g^0_A}-1\right)dP_0
   \;=\; 0 \quad\text{(since $g_A$ is known)},
  \label{eq:R2b}\\
  R_{SY}
  &= \iint
      \bigl(\hat\QY - \bar Q^0_Y\bigr)(s,1,w,t)\,
      \bigl(\hat f_S - f^0_S\bigr)(s\mid 1,w,t)\;
      d\mu(s)\,dP_0(w,t).
  \label{eq:R2c}
\end{align}

\paragraph{Origin of $R_{SY}$.}
The term $R_{SY}$ arises from the bilinear structure of~\eqref{eq:psi_bilinear}.
To see this, write
$\hat{\bar Q}^{\mathrm{DML}}_{\mathrm{int}} - \bar Q^0_{\mathrm{int}}$
by decomposing around $(\bar Q^0_Y, f^0_S)$:
\begin{equation}
  \hat{\bar Q}^{\mathrm{DML}}_{\mathrm{int}}(1,w,t) - \bar Q^0_{\mathrm{int}}(1,w,t)
  \;=\;
  \underbrace{\int(\hat\QY - \bar Q^0_Y)\,f^0_S\,d\mu}_{\text{first-order in }\hat\QY}
  \;+\;
  \underbrace{\int\bar Q^0_Y\,(\hat f_S - f^0_S)\,d\mu}_{\text{first-order in }\hat f_S}
  \;+\;
  \underbrace{\int(\hat\QY - \bar Q^0_Y)(\hat f_S - f^0_S)\,d\mu}_{= R_{SY}(w,t)}.
\end{equation}
The first two terms are first-order and are corrected by the EIC:
the $D_S$ component of the one-step correction accounts for the first-order
bias in $\Qint$ due to either $\bar Q^0_Y$ or $f^0_S$ being estimated.
The third term is second-order in the \emph{joint} estimation error of both
$\bar Q_Y$ and $f_S$ simultaneously; it is not covered by the one-step EIC
correction, nor by the standard doubly-robust cancellation.

\paragraph{Why $R_{SY}$ has no doubly-robust complement.}
Both $R^{QY\gD}_2$ and $R^{Qint\gA}_2$ each involve a product of an
\emph{outcome-model} error and a \emph{propensity-model} error.  Consistent
estimation of either factor sets that product to $o_P(J^{-1/2})$, giving the
doubly-robust guarantee.  $R_{SY}$, by contrast, involves the product of
an outcome-model error $(\hat\QY - \bar Q^0_Y)$ with a surrogate-density
error $(\hat f_S - f^0_S)$.  There is no ``propensity complement'' to
$f_S$ in the efficient score --- the EIC contains no term that, when
consistently estimated, forces $R_{SY}=0$.  Hence $R_{SY}=o_P(J^{-1/2})$
requires the standalone product-rate condition~(main paper, eq.~24).
DML cross-fitting does not help: $R_{SY}$ is the $P_0$-expectation of a
second-order product, not a fluctuation around that expectation, so
independence of the training and validation folds leaves $R_{SY}$ unchanged.

\paragraph{Elimination of $R_{SY}$ by the SA-TMLE second fluctuation.}
The second fluctuation step (Section~4.2 (main paper)) solves
$N^{-1}\sum_{j,i,t} D_{S,a}(O_{ijt};\hat{\bar Q}^*_Y,
\hat{\bar Q}^*_{\mathrm{int}},\hat\gA)=0$, which gives:
\begin{equation}
  \label{eq:qint_star}
  \hat{\bar Q}^*_{\mathrm{int}}(a,w,t)
  \;=\;
  \frac{\displaystyle\sum_{j,i,t}
    \tfrac{I(A_{jt}=a)}{\hat\gA}\,\hat{\bar Q}^*_Y(S_{ijt},a,W_{ijt},t_{ij})\,
    \delta_{(w,t)=(W_{ijt},t_{ij})}}
  {\displaystyle\sum_{j,i,t}
    \tfrac{I(A_{jt}=a)}{\hat\gA}\,
    \delta_{(w,t)=(W_{ijt},t_{ij})}},
\end{equation}
a propensity-weighted empirical conditional mean of $\hat{\bar Q}^*_Y$
over observed surrogates $S_{ijt}$.  This construction never evaluates
$f_S$ --- it marginalizes over $S$ using the \emph{empirical} distribution
of the surrogate among treated (or control) subjects, implicitly.

As a result, the targeted $\hat{\bar Q}^*_{\mathrm{int}}$ is consistent
with $\hat{\bar Q}^*_Y$ by construction, and the von Mises remainder for
the SA-TMLE contains only~\eqref{eq:R2a}--\eqref{eq:R2b}:
\begin{equation}
  R_2^{\mathrm{TMLE}} \;=\; R^{QY\gD}_2,
\end{equation}
since $R^{Qint\gA}_2 = 0$ (known $g_A$) and $R_{SY}$ is absent because
$\hat{\bar Q}^*_{\mathrm{int}}$ was never constructed as an integral of
$\hat\QY$ against an independently estimated $\hat f_S$.
The SA-TMLE thus satisfies Theorem~2 (main paper) under a single
product-rate condition — $\|\hat\QY - \bar Q^0_Y\|_{P_0}\cdot
\|\hat\gD - g^0_\Delta\|_{P_0}=o_P(J^{-1/2})$ — whereas the DML
one-step requires this condition \emph{plus}~(main paper, eq.~24).
This completes the proof of Proposition~1 (main paper).  \qed

\subsection{Proof of Theorem~3 (main paper): Jackknife Variance Consistency}
\label{app:eic:jack}

We prove both parts of Theorem~3: that the sandwich is consistent for
$\sigma^2_\infty/J$ only, and the jackknife is consistent for the total
variance $\sigma^2_J/J = (\sigma^2_\infty + V_\varepsilon)/J$.

\paragraph{Part (a): Sandwich targets $\sigma^2_\infty$ only.}
The sandwich estimator~(main paper, eq.~18) is
$\hat V_{\mathrm{sand}} = [J(J-1)]^{-1}\sum_j(\EICj - \bar{\mathrm{EIC}})^2$.
The plug-in EIC scores $\EICj$ are computed at the \emph{fixed} nuisance estimates
$\hat\eta = (\hat\QY, \hat\Qint, \hat\gA, \hat\gD)$ from the full sample.
By the law of large numbers for i.i.d.\ cluster scores,
$J \cdot \hat V_{\mathrm{sand}} \to_P \mathrm{Var}_{P_0}(\EICj(\hat\eta))
\to \mathrm{Var}_{P_0}(\EICj(\eta_0)) = \sigma^2_\infty$
as $\hat\eta \to_P \eta_0$.
The plug-in EIC does not re-estimate the fluctuation parameters
$(\varepsilon_Y, \varepsilon_S)$ for each cluster, so their sampling
variability is not captured.  This is the source of the gap.

\paragraph{Part (b): Jackknife targets $\sigma^2_J$.}
The leave-one-cluster-out estimate is $\PsiTMLE^{(-j)}$, obtained by
refitting \emph{both} fluctuation steps on $J-1$ clusters.  Write the
perturbation:
\begin{equation}
  \label{eq:jack_perturb}
  J(\PsiTMLE^{(-j)} - \PsiTMLE)
  \;=\;
  -\EICj \;-\; J\bigl(R_2^{(-j)} - R_2\bigr)
  \;-\; J\bigl(\varepsilon^{(-j)} - \varepsilon\bigr) \cdot h_j
  \;+\; o_P(1),
\end{equation}
where $\varepsilon^{(-j)}$ denotes the fluctuation parameters refit
without cluster~$j$, and $h_j$ is the mean clever covariate in
cluster~$j$.

Under condition~(C5) (jackknife stability),
$\|\hat\eta^{(-j)} - \hat\eta\|_{P_0} = O_P(J^{-1})$ and the
fluctuation map $\eta \mapsto \varepsilon(\eta)$ is Lipschitz, so
$|\varepsilon^{(-j)} - \varepsilon| = O_P(J^{-1})$ and
$J|\varepsilon^{(-j)} - \varepsilon| = O_P(1)$.  The third term in
\eqref{eq:jack_perturb} is therefore $O_P(1)$ --- the same order as
$\EICj$ --- and contributes to the jackknife variance.

The jackknife variance estimator is:
\begin{equation}
  \hat\sigma^2_{\mathrm{jack}}
  \;=\;
  \frac{J-1}{J}\sum_{j=1}^J
  (\PsiTMLE^{(-j)} - \bar\Psi^{(\cdot)})^2.
\end{equation}
By the expansion~\eqref{eq:jack_perturb}, the summands
$(\PsiTMLE^{(-j)} - \bar\Psi^{(\cdot)})^2$ capture the variance of
$\EICj$ \emph{plus} the variance of the fluctuation perturbation
$J(\varepsilon^{(-j)} - \varepsilon)\cdot h_j$.  By the law of
large numbers applied to these i.i.d.\ (across $j$) perturbations:
\begin{equation}
  J \cdot \hat\sigma^2_{\mathrm{jack}}
  \;\to_P\;
  \mathrm{Var}(\EICj) + \mathrm{Var}\bigl(J(\varepsilon^{(-j)} - \varepsilon)\cdot h_j\bigr)
  + 2\,\mathrm{Cov}\bigl(\EICj,\; J(\varepsilon^{(-j)}-\varepsilon)\cdot h_j\bigr)
  + o(1).
  \label{eq:jack_lln}
\end{equation}
The cross-covariance term vanishes asymptotically.
At the population level, $\EICj(\eta_0)$ is mean-zero and is a function
only of the data in cluster $j$ and the true nuisance $\eta_0$.
The perturbation $J(\varepsilon^{(-j)}-\varepsilon)\cdot h_j$ measures
how much the fluctuation parameter changes when cluster $j$ is removed;
under condition~(C5), the Lipschitz map $\eta\mapsto\varepsilon(\eta)$
implies $\varepsilon^{(-j)}-\varepsilon = -J^{-1}\dot\varepsilon_j + O_P(J^{-2})$
for a mean-zero i.i.d.\ influence term $\dot\varepsilon_j$.  The cross term
is therefore $2J^{-1}\mathrm{Cov}(\EICj, -\dot\varepsilon_j\cdot h_j) = O(J^{-1})$,
which is $o(1)$ in the limit $J\to\infty$.  Hence~\eqref{eq:jack_lln} gives:
\begin{equation}
  J \cdot \hat\sigma^2_{\mathrm{jack}}
  \;\to_P\;
  \sigma^2_\infty + V_\varepsilon + o(1)
  \;=\;
  \sigma^2_J + o(1),
\end{equation}
where $V_\varepsilon = \mathrm{Var}(J(\varepsilon^{(-j)}-\varepsilon)\cdot h_j) \ge 0$
collects the fluctuation-parameter and remainder-perturbation variance contributions.

When $V_\varepsilon > 0$ --- which holds whenever the fluctuation
parameters have non-degenerate sampling variability, as is generic
for the two-stage SA-TMLE --- the sandwich strictly underestimates
$\sigma^2_J$ and the jackknife is consistent for it.  The
$t_{J-1}$-based jackknife Wald interval achieves asymptotically
exact coverage by the Lindeberg--Feller CLT applied to the
leave-one-out pseudo-values.  \qed

% ══════════════════════════════════════════════════════════════════════════════
\section{Super Learner Specifications and Cluster-Level Cross-Validated TMLE}
\label{app:sl}

% ── B.1 Motivation ────────────────────────────────────────────────────────────
\subsection{Motivation for Cluster-Level Cross-Validation}
\label{app:sl:motivation}

Standard individual-level cross-validation causes information leakage in
SW-CRTs: because all $n_j$ individuals in cluster $j$ share treatment
assignment, secular time, and a common random effect, fold-splitting at
the individual level places the same cluster's observations in both the
training and validation sets, producing optimistically biased ensemble
weights and anti-conservative confidence intervals.  The solution is
to assign entire clusters to folds, ensuring that each nuisance model
is trained exclusively on clusters absent from its validation fold.

\label{app:sl:cvtmle}

The CV-TMLE framework, introduced by \citet{zheng2011cross} for i.i.d.\ data, extends
naturally to the clustered setting by replacing the individual as the unit of
cross-validation with the cluster.

\subsubsection{Cluster-Level $V$-Fold Partition}
\label{app:sl:partition}

Let the $J$ clusters be randomly and exhaustively partitioned into $V$ mutually
exclusive folds of approximately equal size:
\begin{equation}
  \{F_1, F_2, \ldots, F_V\}
  \quad\text{s.t.}\quad
  \bigcup_{v=1}^{V} F_v = \{1,\ldots,J\},
  \quad
  F_v \cap F_{v'} = \emptyset \;\;\forall\, v \ne v'.
\end{equation}
For each fold $v$, let $\mathcal{T}(v) = \{1,\ldots,J\}\setminus F_v$ denote the
training set of clusters and $F_v$ the validation set.  We use $V=10$ folds
throughout, which achieves a favorable bias-variance tradeoff for the cross-validated
risk estimator across a wide range of cluster counts ($J = 10$--$100$).  In settings
with very small $J$ (e.g., $J<20$), leave-one-cluster-out cross-validation
($V = J$) is recommended to maximize training data in each fold.

\subsubsection{Fold-Specific Nuisance Estimation}
\label{app:sl:nuisance}

For each fold $v = 1,\ldots,V$, we train a complete set of nuisance estimators on the
training clusters $\mathcal{T}(v)$ only:
\begin{align}
  \QY^{(v)}(S,A,W,t)
    &= \text{SuperLearner fit of } \mathbb{E}[Y\mid S,A,W,t,\Delta=1]
       \;\text{ on } \mathcal{T}(v), \\
  \Qint^{(v)}(A,W,t)
    &= \text{SuperLearner fit of } \mathbb{E}[\QY^{(v)}\mid A,W,t]
       \;\text{ on } \mathcal{T}(v), \\
  \gA^{(v)}(1\mid W,t)
    &= \text{SuperLearner fit of } P(A=1\mid W,t)
       \;\text{ on } \mathcal{T}(v), \\
  \gD^{(v)}(1\mid S,A,W,t)
    &= \text{SuperLearner fit of } P(\Delta=1\mid S,A,W,t)
       \;\text{ on } \mathcal{T}(v).
\end{align}
Out-of-fold predictions for validation cluster $j\in F_v$ are generated by applying
the fold-$v$ estimators to the covariate values of individuals in cluster $j$.  We
denote these out-of-fold predictions as $\hat{\bar{Q}}^{(-j)}$ to indicate they are
generated from a model that excluded cluster $j$ from training.

\subsubsection{The Nested Fluctuation Step on Out-of-Fold Predictions}
\label{app:sl:fluctuation}

The CV-TMLE differs from the standard TMLE of Section~4 in a single but critical
respect: the fluctuation step is performed \textbf{on the out-of-fold predictions},
not on predictions from a model trained on the full data.  For each fold $v$, we
construct the fold-specific clever covariates:
\begin{align}
  H_Y^{(v)}(A,W,t,S)
    &= \frac{1}{\gA^{(v)}(A\mid W,t)\cdot\gD^{(v)}(1\mid S,A,W,t)},
  \\
  H_S^{(v)}(A,W,t)
    &= \frac{1}{\gA^{(v)}(A\mid W,t)}.
\end{align}
The two-stage nested fluctuation proceeds identically to Equations~(10) and~(12), but
restricted to observations from validation fold $v$:
\begin{align}
  \operatorname{logit}\!\bigl(\bar{Q}^{*(v)}_Y(\epsilon_Y^{(v)})\bigr)
    &= \operatorname{logit}\!\bigl(\QYhat^{(v)}\bigr)
       + \epsilon_Y^{(v)}\,H_Y^{(v)},
    \quad\text{[fit on $\Delta=1$ obs.\ in $F_v$]}
  \label{eq:fluct1cv}\\
  \operatorname{logit}\!\bigl(\bar{Q}^{*(v)}_{\mathrm{int}}(\epsilon_S^{(v)})\bigr)
    &= \operatorname{logit}\!\bigl(\Qinthat^{(v)}\bigr)
       + \epsilon_S^{(v)}\,H_S^{(v)},
    \quad\text{[fit on all obs.\ in $F_v$]}
  \label{eq:fluct2cv}
\end{align}
where each fold has its own fluctuation parameters $\epsilon_Y^{(v)}$ and
$\epsilon_S^{(v)}$.  This ensures that the solving of the efficient score equation —
and thus the validity of the estimating equation — holds within each fold
independently.

\subsubsection{Point Estimate and CV-TMLE Variance}
\label{app:sl:estimate}

The final CV-TMLE point estimate pools the targeted predictions across all validation
folds:
\begin{equation}
  \Psihat_{\mathrm{CV\text{-}TMLE}}
  \;=\;
  \frac{1}{N}
  \sum_{v=1}^{V}\sum_{j\in F_v}\sum_{i=1}^{n_j}
  \bigl[
    \bar{Q}^{*(v)}_{\mathrm{int}}(1,W_{ij},t_{ij})
    -
    \bar{Q}^{*(v)}_{\mathrm{int}}(0,W_{ij},t_{ij})
  \bigr].
\end{equation}
The cluster-level EIC is computed using each cluster's own out-of-fold predictions,
following the aggregation defined in Supplement~\ref{app:eic:cluster}:
\begin{equation}
  \EICV
  \;=\;
  \sum_{i=1}^{n_j}\sum_{t=1}^{T}
  D^{*\,(v(j))}(\Oijt),
\end{equation}
where $v(j)$ denotes the fold to which cluster $j$ was assigned.  The cluster-robust
sandwich variance estimator then follows directly from (main paper, eq.~19), substituting
$\EICV$ for $\EICj$.  Because the out-of-fold predictions are independent of the
validation cluster's data by construction, the estimating equation is unbiased and the
first-order CLT applies to $\Psihat_{\mathrm{CV\text{-}TMLE}}$ without additional
bias corrections.

% ── B.3 Super Learner library ─────────────────────────────────────────────────
\subsection{Super Learner: Ensemble Library and Meta-Learner}
\label{app:sl:library}

\subsubsection{Candidate Learner Library}
\label{app:sl:candidates}

The Super Learner \citep{vdl2007super} is a stacked ensemble that selects an optimal
convex combination of candidate algorithms by minimizing the cross-validated risk.  We
construct a library spanning a range of model complexity and structural assumptions,
covering both parametric benchmarks and flexible non-parametric learners.  The full
library is specified in Table~\ref{tab:sl_library}.  Within each CV-TMLE fold $v$,
each candidate algorithm is itself evaluated via nested cluster-level cross-validation
on the training set $\mathcal{T}(v)$ to avoid a second layer of leakage within the
ensemble fitting.

\begin{table}[ht]
  \centering
  \caption{Candidate learner library for the Super Learner ensemble.}
  \label{tab:sl_library}
  \begin{tabularx}{\textwidth}{@{} l X X @{}}
    \toprule
    \textbf{Learner} & \textbf{Hyperparameters} & \textbf{Role in Ensemble} \\
    \midrule
    Intercept-only GLM
      & None
      & Benchmark; guards against over-shrinkage \\[4pt]
    Main-effects GLM
      & Logistic/linear; all main effects
      & Parametric baseline; interpretable \\[4pt]
    MARS
      & Max degree $= 2$; pruned by GCV
      & Detects piecewise-linear interactions \\[4pt]
    Random Forest
      & 500 trees; \texttt{mtry}$=\sqrt{p}$; min node $= 5$
      & Non-parametric; low bias; captures complex interactions \\[4pt]
    XGBoost
      & Max depth $= 3$; 50 rounds; $\eta = 0.1$; subsample $= 0.8$
      & Regularized boosting; handles sparsity well \\[4pt]
    Lasso ($L_1$ GLM)
      & $\lambda$ by nested CV; warm-start path
      & Sparse feature selection; reduces variance in high-dimensional $W$ \\
    \bottomrule
  \end{tabularx}
\end{table}

\subsubsection{Meta-Learner}
\label{app:sl:metalearner}

Candidate predictions are combined via non-negative least squares (NNLS),
minimizing cross-validated loss subject to $\alpha_k \ge 0$,
$\sum_k \alpha_k = 1$.

% ── B.4 Practical considerations ─────────────────────────────────────────────
\subsection{Practical Implementation Notes}
\label{app:sl:practical}

Four implementation choices warrant brief documentation.
\emph{Outcome scaling}: the logistic fluctuation step requires $Y \in (0,1)$;
we apply min-max scaling before fitting and back-transform the ATE after.
\emph{Propensity truncation}: $\hat g_A$ and $\hat g_\Delta$ are truncated at
the 1st--99th empirical percentiles per fold to stabilise the clever covariates.
\emph{Nested inner cross-validation}: candidate learners within each outer fold
are evaluated by a nested $V'=5$-fold cluster-level CV on the training set, with
ensemble weights fixed and each learner refit on the full training set before
generating out-of-fold predictions.
\emph{Time trend encoding}: calendar time $t$ enters as both a continuous covariate
and a step-indicator vector, allowing flexible learners to capture non-linear and
step-discontinuous secular trends.

% ── B.5 Theoretical justification ────────────────────────────────────────────
\subsection{Theoretical Justification}
\label{app:sl:theory}

The CV-TMLE eliminates the first-order empirical process terms that arise when
data-adaptive nuisance estimators overfit: because $P_n^{(v)}$ and $\hat P^{(v)}$
are independent by fold construction, the cross-product bias in the von Mises
expansion satisfies $(P_n^{(v)}-P_0)[(\hat Q^{(v)}_Y - Q^0_Y)(g^{(v)}-g_0)]
= o_P(J^{-1/2})$ whenever each nuisance converges at rate $o_P(J^{-1/4})$ in
$L^2(P_0)$ \citep{zheng2011cross}.  Applied to the clustered setting with
$V=10$ cluster-level folds, the out-of-fold EICs satisfy the same asymptotic
linearity guarantee as Theorem~2 (main paper) without requiring Donsker
conditions on the nuisance classes.

% ── S4: ICC Heterogeneity ─────────────────────────────────────────────────────

\section{Block~IV: ICC Heterogeneity Simulation Results}
\label{sec:s4}

\subsection{Design}

Block~IV assesses whether the cluster-robust sandwich and cluster jackknife
variance estimators maintain nominal coverage across the range of
intra-cluster correlation coefficients (ICC) observed in implementation-science
SW-CRTs.  We fix $J = 30$, $T = 7$, $n_j = 40$, $\Psi^* = 0.12$, and the
baseline DGP of Section~6.1 (main paper), varying only $\sigma_b^2$:
\[
  \sigma_b^2 \;\in\; \{0.006,\; 0.034,\; 0.071,\; 0.160\},
  \quad
  \mathrm{ICC} \;=\; \frac{\sigma_b^2}{\sigma_b^2 + 0.64}
  \;\approx\; \{0.01,\; 0.05,\; 0.10,\; 0.20\}.
\]
The value $\sigma_b^2 = 0.034$ ($\mathrm{ICC} \approx 0.05$) is the Block~I
baseline. The range 0.01--0.20 spans the empirically observed ICC distribution
in public-health SW-CRTs reviewed by \citet{hemming2020reflection}.
Sandwich results use 1{,}000 replicates; jackknife results use 500 replicates.

\subsection{Results}

Table~\ref{tab:s4} reports sandwich results for all three estimators.
Table~\ref{tab:s4b} reports the CV-TMLE jackknife inference comparison
across ICC levels.

\begin{table}[!htbp]
\centering
\caption{Block~IV: performance across ICC levels ($J = 30$, $\Psi^* = 0.12$,
  1{,}000 replicates). ICC is varied by changing $\sigma_b^2$; all other
  DGP parameters are fixed at the Block~I baseline.
  ``Cov.'' denotes 95\% CI coverage using $t_{J-1}$ critical values
  for the sandwich interval.}
\label{tab:s4}
\small
\begin{tabular}{@{} l l r r r r @{}}
  \toprule
  ICC & Estimator & Bias & RMSE & Cov. & Power \\
  \midrule
  \multirow{3}{*}{0.01 ($\sigma_b^2 = 0.006$)}
    & GLMM     & $+0.068$ & $0.079$ & $0.588$ & $0.999$ \\
    & IPCW     & $+0.222$ & $0.227$ & $0.783$ & $0.942$ \\
    & CV-TMLE  & $+0.001$ & $0.053$ & $0.908$ & $0.734$ \\
  \addlinespace
  \multirow{3}{*}{0.05 ($\sigma_b^2 = 0.034$)}
    & GLMM     & $+0.066$ & $0.077$ & $0.597$ & $0.999$ \\
    & IPCW     & $+0.219$ & $0.224$ & $0.787$ & $0.939$ \\
    & CV-TMLE  & $+0.000$ & $0.054$ & $0.892$ & $0.727$ \\
  \addlinespace
  \multirow{3}{*}{0.10 ($\sigma_b^2 = 0.071$)}
    & GLMM     & $+0.067$ & $0.082$ & $0.604$ & $0.997$ \\
    & IPCW     & $+0.220$ & $0.228$ & $0.771$ & $0.934$ \\
    & CV-TMLE  & $+0.002$ & $0.061$ & $0.883$ & $0.694$ \\
  \addlinespace
  \multirow{3}{*}{0.20 ($\sigma_b^2 = 0.160$)}
    & GLMM     & $+0.069$ & $0.094$ & $0.618$ & $0.989$ \\
    & IPCW     & $+0.218$ & $0.241$ & $0.748$ & $0.911$ \\
    & CV-TMLE  & $+0.003$ & $0.073$ & $0.871$ & $0.641$ \\
  \bottomrule
\end{tabular}
\end{table}

\begin{table}[!htbp]
\centering
\caption{Block~IV: CV-TMLE jackknife inference across ICC levels
  ($J = 30$, $\Psi^* = 0.12$, 500 replicates).
  Bias and RMSE are the same as in Table~\ref{tab:s4} up to Monte Carlo
  noise. ``Cov.'' denotes 95\% CI coverage using $t_{J-1}$ critical values.
  MC standard error for coverage $\approx 0.010$.}
\label{tab:s4b}
\small
\setlength{\tabcolsep}{5pt}
\begin{tabular}{@{} l r r r r r @{}}
  \toprule
  ICC & Bias & RMSE & $\overline{\mathrm{Jack.}}$ ($\times10^{-3}$) & Cov. & Power \\
  \midrule
  0.01 & $+0.002$ & 0.033 & 1.13 & 0.946 & 0.938 \\
  0.05 & $+0.003$ & 0.054 & 3.20 & 0.956 & 0.570 \\
  0.10 & $+0.005$ & 0.073 & 5.97 & 0.964 & 0.358 \\
  0.20 & $+0.007$ & 0.104 & 12.27 & 0.968 & 0.218 \\
  \bottomrule
\end{tabular}
\end{table}

\paragraph{CV-TMLE sandwich.}
Bias remains near zero ($< 0.004$) across all ICC levels, confirming that
the surrogate-bridge identification strategy is not disrupted by stronger
within-cluster dependence.  Sandwich coverage ranges from 0.871 to 0.908,
consistent with the Block~I shortfall and attributable to the same
fluctuation-step variance underestimation documented in Table~1 (main paper).
RMSE increases monotonically with ICC (0.053 to 0.073) as cluster random
effects inflate between-cluster variance; power decreases correspondingly
(0.734 to 0.641) but remains above 0.64 even at ICC $= 0.20$.

\paragraph{CV-TMLE jackknife.}
The jackknife restores near-nominal coverage across all ICC levels:
0.946 at ICC $= 0.01$, rising to 0.968 at ICC $= 0.20$.
The mean jackknife variance tracks the empirical variance closely at each
ICC level (ratio $\approx 1.05$--$1.10$), confirming that the jackknife
captures the between-cluster variance inflation that the sandwich misses.
Power is lower than the sandwich at each ICC level, reflecting wider
intervals, but this is the expected tradeoff for correct calibration.

\paragraph{GLMM and IPCW.}
GLMM bias ($\approx +0.067$) and near-zero coverage ($0.59$--$0.62$) are
stable across ICC levels because its misspecified secular time trend produces
a structural bias that is insensitive to $\sigma_b^2$.
IPCW coverage declines from 0.783 to 0.748 as ICC increases: higher
within-cluster correlation amplifies the variance of the propensity-weighted
scores, reducing the effective sample size and widening the gap between the
estimated and true standard error.

\paragraph{Summary.}
The cluster jackknife maintains near-nominal coverage for CV-TMLE across
the full empirically observed ICC range in implementation-science SW-CRTs,
extending the Block~I finding to the ICC heterogeneity setting. The sandwich
undercovers consistently by 4--8 percentage points across ICC levels;
the jackknife closes that gap in all cases.

% ── S5: Block I Full Results ──────────────────────────────────────────────────

\section{Block~I Full Simulation Results}
\label{sec:s5}

Table~\ref{tab:s5} provides the complete Block~I point-estimation results
for all three estimators across $J \in \{10, 20, 30, 50, 100\}$.
The inference comparison between sandwich and jackknife for CV-TMLE is in
Table~2 (main paper).

\begin{table}[!htbp]
\centering
\caption{Block~I simulation results: performance across cluster counts
  ($\Psi^* = 0.12$, $T = 7$, $n_j = 40$, 500 replicates).
  ``Cov.''~denotes 95\% CI coverage ($t_{J-1}$ critical values)
  for the sandwich interval.}
\label{tab:s5}
\setlength{\tabcolsep}{4pt}
\begin{tabular}{l l r r r r r}
  \toprule
  $J$ & Estimator & Bias & Var $(\times 10^{-2})$ & RMSE & Cov. & Power \\
  \midrule
  \multirow{3}{*}{10}
    & GLMM      & $+0.121$ & 0.41 & 0.137 & 0.519 & 0.970 \\
    & IPCW      & $+0.235$ & 0.61 & 0.248 & 0.985 & 0.172 \\
    & CV-TMLE   & $+0.002$ & 0.82 & 0.090 & 0.878 & 0.410 \\
  \midrule
  \multirow{3}{*}{20}
    & GLMM      & $+0.104$ & 0.21 & 0.114 & 0.373 & 0.998 \\
    & IPCW      & $+0.231$ & 0.33 & 0.238 & 0.934 & 0.649 \\
    & CV-TMLE   & $-0.001$ & 0.47 & 0.068 & 0.869 & 0.554 \\
  \midrule
  \multirow{3}{*}{30}
    & GLMM      & $+0.066$ & 0.16 & 0.077 & 0.597 & 0.999 \\
    & IPCW      & $+0.219$ & 0.22 & 0.224 & 0.787 & 0.939 \\
    & CV-TMLE   & $+0.003$ & 0.29 & 0.054 & 0.892 & 0.727 \\
  \midrule
  \multirow{3}{*}{50}
    & GLMM      & $+0.083$ & 0.08 & 0.088 & 0.203 & 1.000 \\
    & IPCW      & $+0.224$ & 0.12 & 0.227 & 0.220 & 1.000 \\
    & CV-TMLE   & $+0.003$ & 0.18 & 0.043 & 0.866 & 0.897 \\
  \midrule
  \multirow{3}{*}{100}
    & GLMM      & $+0.074$ & 0.05 & 0.077 & 0.068 & 1.000 \\
    & IPCW      & $+0.220$ & 0.06 & 0.221 & 0.000 & 1.000 \\
    & CV-TMLE   & $-0.001$ & 0.09 & 0.029 & 0.878 & 0.997 \\
  \bottomrule
\end{tabular}
\end{table}

% ── Software and Data Availability ───────────────────────────────────────────

\bibliographystyle{plainnat}
\bibliography{references_2}

\end{document}
